# Supplementary material for: A Predictive Momentum-Based Whole-Body Torque Controller: Theory and Simulations for the iCub Stepping
Source: arXiv:1705.10635 source file (2017-07-28)
Supplement: Supplementary file 1 [file appendix.tex]

%!TEX root = ../steprecovery.tex
% \appendix
